# Supplementary material for: Attribute Privacy: Framework and Mechanisms
Source: arXiv:2009.04013 source file (2021-05-11)
Supplement: Supplementary file 1 [file appendix.tex]

\input{wassersteinmech}
